# Supplementary material for: Ion heating and flow driven by an Instability found in Plasma Couette Flow
Source: arXiv:2103.12657 ancillary file (2021-03-23)
Supplement: Supplementary file 1 [file Supplemental_Derivation.pdf]

# Supplemental Material for: Instability, ion heating and flow drive in High- $\beta$ Hall Plasmas on the PCX

J. Milhone,<sup>1</sup> K. Flanagan,<sup>1</sup> J. Egedal,<sup>1</sup> D. Endrizzi,<sup>1</sup> J. Olson,<sup>1</sup> E. E. Peterson,<sup>2</sup> R. Sassella,<sup>1</sup> and C. B. Forest<sup>1</sup>

<sup>1</sup>*Department of Physics, University of Wisconsin–Madison,  
1150 University Avenue, Madison, WI 53706, USA*

<sup>2</sup>*Plasma Science and Fusion Center, Massachusetts Institute of Technology,  
77 Massachusetts Avenue, NW 17 Cambridge, MA 02139*

(Dated: March 23, 2021)

Fluctuations from the electromagnetic gradient drift instability have been observed on the Plasma Couette Experiment. Measurements from the experiment indicate the stability is related to the plasma  $\beta$ . We believe this instability is related to the gradient drift instability [1], an electrostatic instability driven by  $\nabla B_z$  and  $\nabla n$  with wavevector perpendicular to  $\hat{z}$ . In addition to density and electrostatic fluctuations, large  $B_z$  fluctuations are observed and require additional physics added to the gradient drift instability to explain the behavior.

The analysis outlined in section II of Frias et al. is extended for magnetic fluctuations in  $B_z$  with wavevector,  $k$ , perpendicular to the applied magnetic field ( $z$ ). The ions are unmagnetized and only follow a ballistic response. The ion continuity equation and momentum equation are

$$\frac{\partial n}{\partial t} + \nabla \cdot (n \mathbf{V}_i) = 0 \quad (1)$$

$$nm_i \left( \frac{\partial \mathbf{V}_i}{\partial t} + (\mathbf{V}_i \cdot \nabla) \mathbf{V}_i \right) = ne\mathbf{E} - T_i \nabla n \quad (2)$$

where the Lorentz force has been neglected because the ions are unmagnetized and the ion temperature is treated as a constant. We assume a Fourier solution  $\sim e^{i(-\omega t + \mathbf{k} \cdot \mathbf{r})}$  for the linear perturbations and assume a Boussinesque approximation ( $k_x L_x \gg 1$ ). With the assumed form, ion continuity and momentum balance become

$$-i\omega \tilde{n} + i\mathbf{k} \cdot \mathbf{V}_{i0} \tilde{n} + in_0 \mathbf{k} \cdot \tilde{\mathbf{V}}_i = 0 \quad (3)$$

$$-i\omega \tilde{\mathbf{V}}_i + i(\mathbf{k} \cdot \mathbf{V}_{i0}) \tilde{\mathbf{V}}_i = -i\mathbf{k} \frac{e\tilde{\Phi}}{m_i} - iV_{thi}^2 \mathbf{k} \frac{\tilde{n}}{n_0} \quad (4)$$

where fluctuating quantities are indicated with a  $\tilde{\phantom{x}}$  and the electric field has been substituted with the electric potential. Combining these two expressions yields a relationship between the density and electric potential fluctuations given by

$$\frac{\tilde{n}}{n_0} = \frac{k_\perp^2}{(\omega - \mathbf{k} \cdot \mathbf{V}_{i0})^2 - k_\perp^2 V_{thi}^2} \frac{e\tilde{\Phi}}{m_i} \quad (5)$$

For fluid theory to be valid,  $\omega - \mathbf{k} \cdot \mathbf{V}_{i0} \gg k_\perp V_{thi}$ , so the  $k_\perp^2 V_{thi}^2$  term is neglected in the analysis.

The electrons are magnetized and have equilibrium  $\mathbf{E} \times \mathbf{B}$  and diamagnetic drift velocities that are compressible which are accounted for when combining the continuity and momentum equations giving

$$\frac{\partial n}{\partial t} + \mathbf{v}_E \cdot \nabla n - 2n(\mathbf{v}_E + \mathbf{v}_{pe}) \cdot \nabla \ln B = 0 \quad (6)$$

where  $v_E$  is the  $\mathbf{E} \times \mathbf{B}$  drift and  $v_{pe}$  is the electron diamagnetic drift. Assuming a Fourier form again, careful linearization of the the drift velocities with the inclusion of magnetic fluctuations gives

$$\tilde{\mathbf{v}}_e = -ik_\phi \frac{\tilde{\Phi}}{B_0} \hat{r} + \left( ik_r \frac{\tilde{\Phi}}{B_0} - u_0 \frac{\tilde{B}}{B_0} \right) \hat{\phi} \quad (7)$$

$$\tilde{\mathbf{v}}_{pe} = ik_\phi \frac{T_e}{eB_0} \frac{\tilde{n}}{n_0} \hat{r} - \left[ \left( ik_r \frac{T_e}{eB_0} + v_* \right) \frac{\tilde{n}}{n_0} + v_* \frac{\tilde{B}}{B_0} \right] \hat{\phi} \quad (8)$$

where  $\mathbf{u}_0 = -E_{r0}/B_0 \hat{\phi}$  is the equilibrium  $\mathbf{E} \times \mathbf{B}$  drift velocity and  $\mathbf{v}_* = -T_e \kappa_n / (eB_0) \hat{\phi}$  is the equilibrium diamagnetic drift with inverse gradient length scale,  $\kappa_n = \partial \ln n / \partial r$ .

The magnetic fluctuations can be related to the density and electric field perturbations through Ampère's Law. Assuming the toroidal current is only from the electron drift velocities and neglecting the displacement current, the radial component of Ampère's law is

$$(\nabla \times \mathbf{B})_r = \mu_0 J_r = -\mu_0 n e \mathbf{V}_e \cdot \hat{\mathbf{r}} \quad (9)$$

where  $\mathbf{V}_e$  is the total electron drift velocity. Linearizing Eq. 9 and inserting Eqns 7-8 gives

$$\frac{\tilde{B}}{B_0} = \frac{\beta}{2} \left( \frac{e\tilde{\Phi}}{T_e} - \frac{\tilde{n}}{n_0} \right) \quad (10)$$

where  $\beta = 2\mu_0 n_0 T_e / B_0^2$  is the electron plasma pressure to magnetic pressure ratio.

Linearizing Eq. 6 and assuming a Fourier solution gives

$$-i\omega\tilde{n} + (\tilde{\mathbf{V}}_E \cdot \hat{\mathbf{r}}) \frac{\partial n_0}{\partial r} + iu_0 k_\phi \tilde{n} - 2n_0 \kappa_B (\tilde{\mathbf{V}}_E + \tilde{\mathbf{V}}_{pe}) \cdot \hat{\mathbf{r}} - 2n_0 (u_0 + v_*) i k_\phi \frac{\tilde{B}}{B_0} = 0 \quad (11)$$

and combining Eqns. 7-10 results in

$$\frac{\tilde{n}}{n_0} = \frac{(1 - \beta)v_* - v_D - \beta v_E}{(\omega/k_\phi) - (1 + \beta)v_E - v_D - \beta v_*} \frac{e\tilde{\Phi}}{T_e} \quad (12)$$

where  $v_D = -2T_e \kappa_B / (eB_0)$  is the electron magnetic drift velocity and  $\kappa_B = \partial \ln B / \partial r$  is the inverse gradient length scale for the magnetic field. Setting  $\beta = 0$  recovers the result from Frias et al. Eq. 16 [1].

Invoking quasi-neutrality to combine Eqns. 5 and 12 gives the dispersion relation

$$\omega = \mathbf{k}_\perp \cdot \mathbf{V}_{io} + \frac{1}{2} \frac{k_\perp^2}{k_\phi} \frac{C_s^2}{\mathcal{A}} \left( 1 \pm \sqrt{1 - 4 \frac{k_\phi^2}{k^2} \frac{\mathcal{A}}{C_s^2} (\mathcal{B} - V_0)} \right) \quad (13)$$

where  $\mathcal{A}$  and  $\mathcal{B}$  are given by

$$\mathcal{A} = (1 - \beta)v_* - v_D - \beta v_E \quad (14)$$

$$\mathcal{B} = (1 + \beta)v_E + v_D + \beta v_* \quad (15)$$

For  $\beta = 0$ , the unstable criterion from Frias et al. is recovered. The condition for instability is

$$\mathcal{A}(\mathcal{B} - V_0) > \frac{1}{4} \frac{k_\perp^2}{k_\phi^2} C_s^2 \quad (16)$$

Assuming  $V_0$  is small and inserting Eqns 14 and 15 gives

$$\left[ (1 - \beta)\kappa_n - 2\kappa_B - \beta \frac{eE_0}{T_e} \right] \left[ (1 + \beta) \frac{eE_0}{T_e} + 2\kappa_B - \beta\kappa_n \right] > \frac{1}{4} \frac{k_\perp^2}{k_\phi^2} \frac{1}{\rho_s^2} \quad (17)$$

where  $\rho_s = C_s / \Omega_{ci}$  is the ion Larmor sound radius.

---

[1] W. Frias, A. I. Smolyakov, I. D. Kaganovich, and Y. Raitses, Long wavelength gradient drift instability in Hall plasma devices. I. Fluid theory, *Physics of Plasmas* **19**, 072112 (2012).
